# Supplementary material for: Marked Neural Spatio-Temporal Point Process Involving a Dynamic Graph Neural Network
Source: arXiv:2206.03469 source file (2024-08-28)
Supplement: Supplementary file 2 [file hyperparameter_tuning.tex]

\subsection{Hyperparameter Tuning}
